# Supplementary material for: Functional metamirrors
Source: arXiv:1411.5559 source file (2014-11-20)
Supplement: Supplementary file 1 [file Supplementary_materials.pdf]

**Supplementary Note 1. Inclusions of the proposed metamirrors.**

In order to ensure full control over reflected wave phase, we exploit inclusions possessing both electric and magnetic response, as well as magnetoelectric coupling. Such properties can be achieved in particular with copper inclusions shown in Fig. S1. They incorporate electrically polarizable straight wires (with the lengths $l_1$ and $l_2$) connected to magnetically polarizable wire loops (with the radii $R_1$ and $R_2$). An external electric field along the $x$-axis excites an electric dipole moment in the straight wires. Moreover, due to the connection between the straight wires and the loop, the external electric field excites also a magnetic moment in the loop. This feature of the inclusions is called magnetoelectric coupling, i.e. electric and magnetic responses of the inclusions are coupled. Likewise, an external magnetic field along the $y$-axis excites a magnetic moment in the loop and an electric dipole moment in the straight wires. The magnetoelectric coupling effect opens up an additional degree of freedom for designing metasurfaces with extreme properties, in particular, metamirrors.

The loops of the inclusions, in addition to the magnetic response, are also electrically polarizable along the $x$-axis. Therefore, the electric polarizability of the whole particle equals to either the sum (the inclusion in Fig. S1a) or the difference (the inclusion in Fig. S1b) of the polarizabilities of the straight wire and loop parts, which leads to different electromagnetic response. The inclusions of the first type (Fig. S1a) effectively reflect waves with the phase from $-\pi/2$ to $\pi/2$. The inclusions of the second type (Fig. S1b) allow one to cover the reflected wave phases from $\pi/2$ to $3\pi/2$.

The copper wire of the inclusions has diameter of 0.55 mm. The capacitive gaps $h_1$=0.8 mm and $h_2$=0.4 mm are identical in all the inclusions of the proposed metamirrors. All the other dimensions as well as locations of the inclusions are given in Table S1 and Table S2.

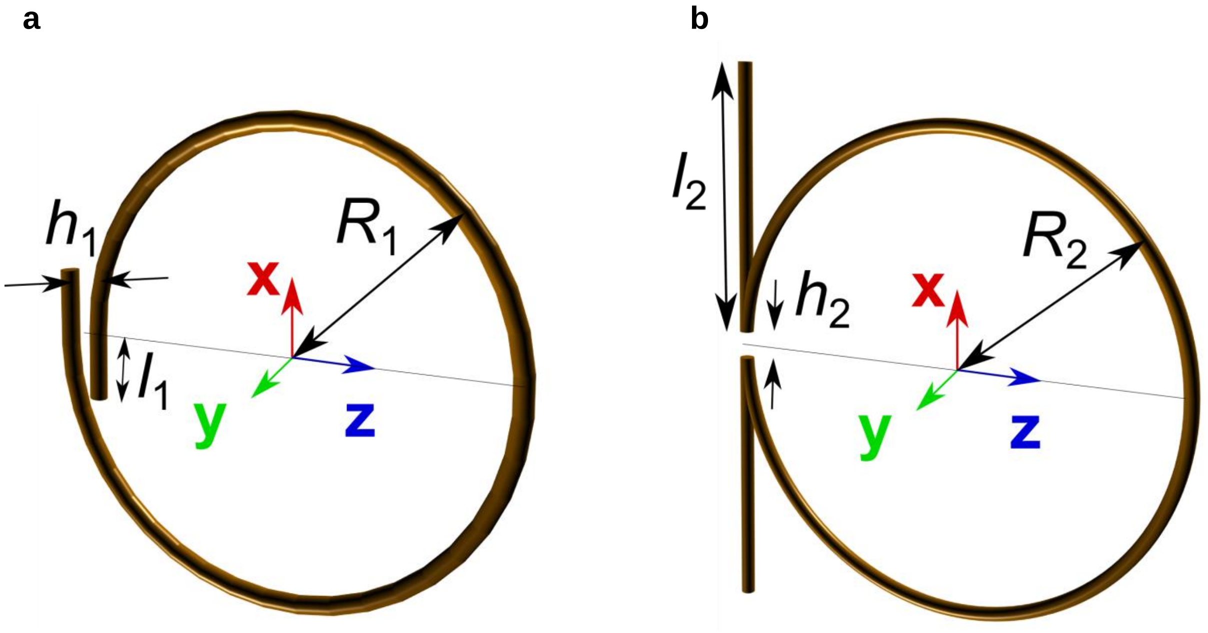


**Supplementary Figure S1 | Metamirror inclusions.** Two types of bianisotropic omega inclusions: (a) So-called twisted omega inclusion (hereinafter, first type); (b) Inclusion with shape of the letter Ω (hereinafter, second type).

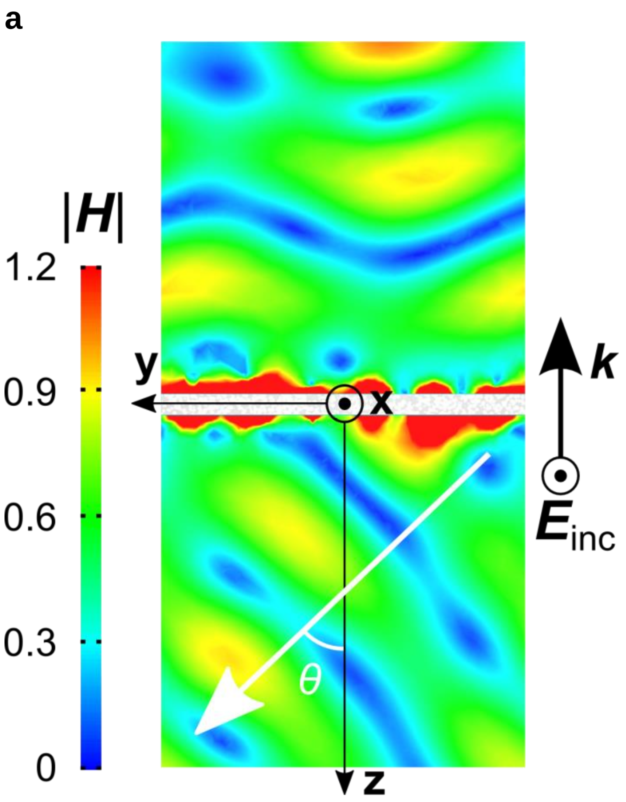


**Supplementary Figure S2 | Frequency stability of the metamirror performance.** (a-b) Magnetic field distribution (normalized to the magnetic field of the incident wave) of the transmitted (the -*z* half-space) and reflected (the +*z* half-space) waves. (a) Operation at 4.87 GHz. (b) Operation at 5.12 GHz.

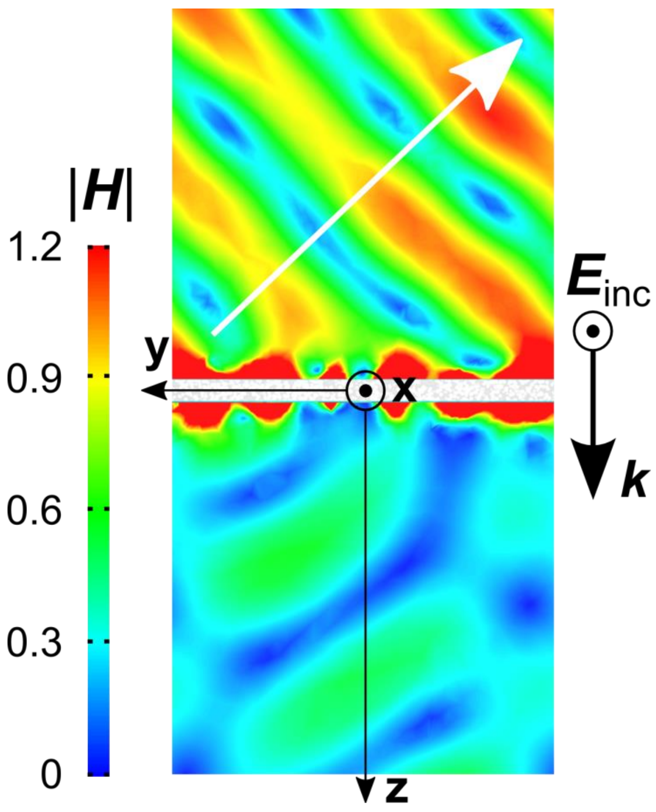


**Supplementary Figure S3 | Operation of the metamirror for illumination from the opposite direction (–*z*-direction).** Magnetic field distribution (normalized to the magnetic field of the incident wave) of the transmitted (the +*z* half-space) and reflected (the -*z* half-space) waves at 5 GHz. The structure operates nearly identically for illumination of its both sides.

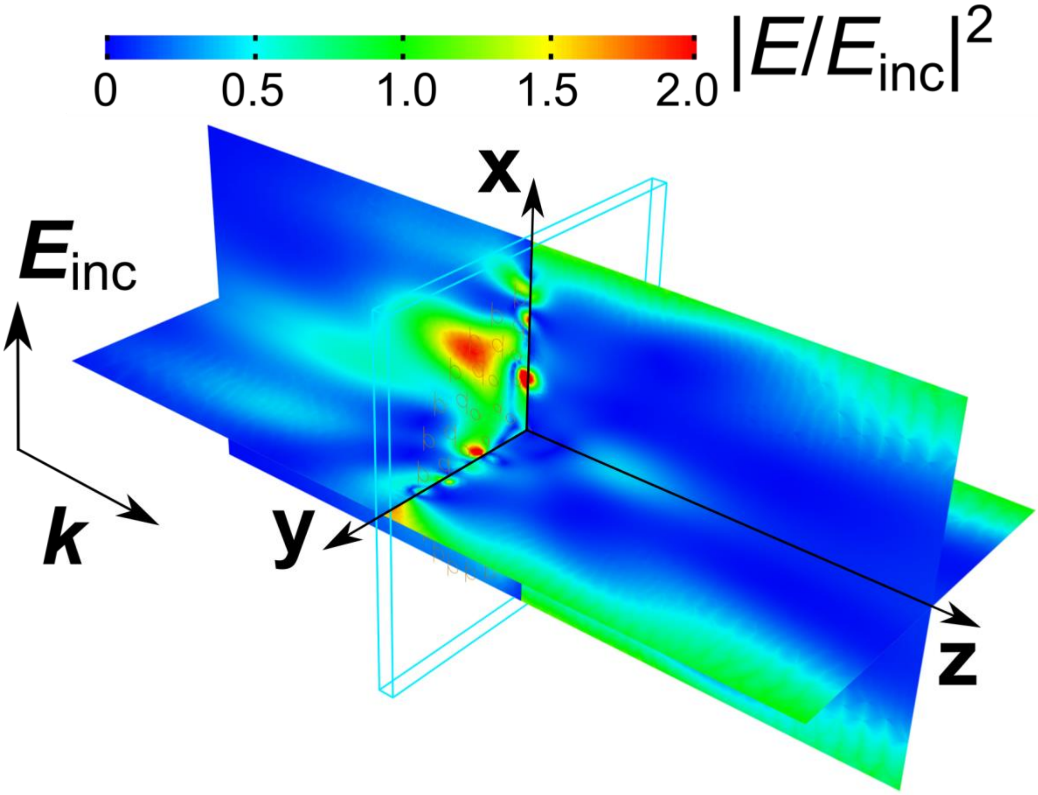


**Supplementary Figure S4 | Operation of the metalens for illumination from the opposite direction (–*z*-direction).** Power density distribution (normalized to the incident power density) of the transmitted (the +*z* half-space) and reflected (the –*z* half-space) waves. The power intensity maps are depicted on two orthogonal cross-section planes (the *xz* and *yz*-planes). The focusing effect is drastically decreased for illumination from the opposite side.

**Supplementary Table S1. Dimensions of the inclusions and their locations within the period of the metamirror.**

| Location along the $y$-axis within the period $d$ | Type of an inclusion | Loop radius, mm | Length of the straight wires, mm | Phase of the backscattered wave |
|---|---|---|---|---|
| $-5d/12$ | First | $R_1$=2.79 | $l_1$=1.29 | 5π/3 |
| $-d/4$ | Second | $R_2$=3.43 | $l_2$=3.49 | 4π/3 |
| $-d/12$ | Second | $R_2$=2.88 | $l_2$=5.42 | π |
| $d/12$ | Second | $R_2$=3.35 | $l_2$=4.01 | 2π/3 |
| $d/4$ | First | $R_1$=3.01 | $l_1$=1.00 | π/3 |
| $5d/12$ | First | $R_1$=2.28 | $l_1$=2.84 | 0 |

**Supplementary Table S2. Dimensions of the inclusions and their locations in the metalens.** The first six inclusions correspond to the inclusions in Fig. 3a.

| Distance to the center of the lens $r$, mm | Type of an inclusion | Loop radius, mm | Length of the straight wires, mm | Phase of the backscattered wave, ° | Position of the straight wires |
|---|---|---|---|---|---|
| 0 | First | $R_1$=3.45 | $l_1$=0.57 | 280 | -$z$ half-space |
| 18 | First | $R_1$=2.66 | $l_1$=1.50 | 306 | -$z$ half-space |
| 33 | First | $R_1$=2.27 | $l_1$=2.87 | 0 | -$z$ half-space |
| 48 | First | $R_1$=3.19 | $l_1$=0.83 | 65 | +$z$ half-space |
| 63 | Second | $R_2$=3.45 | $l_2$=5.26 | 140 | +$z$ half-space |
| 78 | Second | $R_2$=3.49 | $l_2$=5.04 | 218 | -$z$ half-space |
| 93 | First | $R_1$=2.66 | $l_1$=1.50 | 306 | -$z$ half-space |
| 108 | First | $R_1$=2.5 | $l_1$=1.90 | 27 | +$z$ half-space |
| 123 | Second | $R_2$=3.77 | $l_2$=3.55 | 113 | +$z$ half-space |
| 138 | Second | $R_2$=3.33 | $l_2$=5.79 | 207 | -$z$ half-space |
| 153 | First | $R_1$=3.16 | $l_1$=0.88 | 285 | -$z$ half-space |
| 168 | First | $R_1$=2.44 | $l_1$=2.09 | 19 | +$z$ half-space |
